# Supplementary material for: A Finite Element Configuration Interaction Method for Wigner Localization
Source: arXiv:2208.07526 source file (2022-08-16)
Supplement: Supplementary file 1 [file bak-appendix.tex]

% appendix


\section*{Appendix}
\subsubsection*{KS DFT with SCE model}

For the purpose of generalizing the discussion for the strongly correlated electronic systems, we introduce the single partical density:
$$\rho(\mathbf{r})= N\sum_{\sigma_1,\dots,\sigma_N}\int d\mathbf{r}_2\dots d\mathbf{r}_N| \Psi(\mathbf{r},\sigma_1, \dots,\mathbf{r}_N,\sigma_N)|^2,\eqno{(3.2.1)}$$
which is normalized according to $\int \rho(\mathbf{r})d\mathbf{r} = N$. Let this function as the variable, the universal Hohenberg-Kohn (HK) functional of DFT  is defined as [{\color{red}4:30,31}]
 $$F_\alpha [\rho] =\min\limits_{\Psi\mapsto \rho}\langle\Psi|\alpha\hat{T}+\hat{V}_\mathrm{ee}|\Psi\rangle\geq 0,\eqno{(3.2.2)}$$
where the constraint $\Psi\mapsto \rho$ addresses all those wave functions $\Psi$ with the same given density $\rho=\rho(\mathbf{r})$, according to (3.2.1). And the ground state energy of (2.1.9) could be obtained by,
$$E_\alpha = \min\limits_{\rho\mapsto N}\Big\{ F_\alpha[\rho]+\int\rho(\mathbf{r})v(\mathbf{r})d\mathbf{r}\Big\}:=\min\limits_{\rho\mapsto N}E_\alpha [\rho],\eqno{(3.2.3)}$$
where the condition $\rho\mapsto N$ now addresses all (non-negative) density functions $\rho(\mathbf{r})$ that are normalized to the same given particle number $N$.

For a given density $\rho$ and interaction weakness $\alpha$ in (3.2.2), let $\Psi_\alpha [\rho]$ be a minimizing wave function. We define a density $\rho$ to be ground state density if $\Psi_\alpha [\rho]$ is a ground state of $ \hat{H}_\alpha $, and the corresponding ground state energy is
$$E_\alpha [\rho] = F_\alpha[\rho] + \int\rho(\mathbf{r})v(\mathbf{r})d\mathbf{r}.$$



We consider the limit $\alpha \to 0$ of infinitely strong repulsion with a given smooth $N$-electron density $\rho$ [{\color{red}4:39,40}], which be called the ‘‘strictly correlated electroins" (SCE) limit [{\color{red}9}],
$$\lim_{\alpha\to0}F_\alpha[\rho]=\min\limits_{\Psi\mapsto \rho}\langle\Psi|\hat{V}_\mathrm{ee}|\Psi\rangle:= V_\mathrm{ee}^{\mathrm{SCE}}[\rho].\eqno{(3.2.4)}$$
$V_\mathrm{ee}^{\mathrm{SCE}}[\rho]$ introduces a reference system in which the electrons are strictly correlated, in the sense that the position of one of them determines the positions of the others in order to minimize the total Coulomb repulsion  [{\color{red}4}].
And the limiting minimizing
wave function $\Psi^{\mathrm{SCE}}[\rho]$ dosen't depend on the spin variables $\sigma_1,\dots,\sigma_N$, and, since the limit is classical, we can only determine $|\Psi^{\mathrm{SCE}}[\rho]|^2$, which, in terms of the spatial variables $\mathbf{r}_1,\dots,\mathbf{r}_N$, is a Dirac-type distribution,
describing electrons with strictly correlated positions [{\color{red}4,4:40,41}].

\subsubsection*{Semi-numerical prediction of initial guess}
When dealing with the strong correlated systems, HF is not a good initial state because it ignores the correlation of electrons [{\color{red}10}]. Through the characterization of the SCE limit, we could construct a good initial guess.

Firstly, we need to predict the positions of peaks of the ground state density in the SCE system, the corresponding ground state energy is
\begin{equation}
	\begin{aligned}
	E_0:=& \min\limits_{\rho\mapsto N}\lim_{\alpha\to0}E_\alpha [\rho]
	 \notag \\
	 =& \min\limits_{\rho\mapsto N}\lim_{\alpha\to0}\Big\{F_\alpha[\rho] + \int\rho(\mathbf{r})v(\mathbf{r})d\mathbf{r}\Big\}\\
	 =&  \min\limits_{\rho\mapsto N} \Big\{\lim_{\alpha\to0}F_\alpha[\rho] + \int\rho(\mathbf{r})v(\mathbf{r})d\mathbf{r}\Big\}\\
	 =:& \min\limits_{\rho\mapsto N} E_0[\rho].
	\end{aligned}\eqno{(3.2.5)}
\end{equation}
If $\rho$ is a smooth density, then according to (3.2.4),
$$ \lim_{\alpha\to0}F_\alpha[\rho] =\langle\Psi^{\mathrm{SCE}}[\rho]|\hat{V}_\mathrm{ee}|\Psi^{\mathrm{SCE}}[\rho]\rangle,$$
and 
$$ \int\rho(\mathbf{r})v(\mathbf{r})d\mathbf{r}=\langle\Psi^{\mathrm{SCE}}[\rho]|\hat{V}_\mathrm{ext}|\Psi^{\mathrm{SCE}}[\rho]\rangle.$$
We have $$E_0[\rho]=\langle\Psi^{\mathrm{SCE}}[\rho]|\hat{V}_\mathrm{ee}+\hat{V}_\mathrm{ext}|\Psi^{\mathrm{SCE}}[\rho]\rangle.$$
Since $|\Psi^{\mathrm{SCE}}[\rho]|^2$ is only determined by spatial variables, writting $$|\Psi^{\mathrm{SCE}}[\rho]|^2=|\Psi^{\mathrm{SCE}}(\mathbf{r}_1,\dots,\mathbf{r}_N)|^2,$$ we obtain
$$E_0[\rho] =\int|\Psi^{\mathrm{SCE}}(\mathbf{r}_1,\dots,\mathbf{r}_N)|^2\Bigg\{\sum_{i=1}^{N-1}\sum_{j=i+1}^N \frac{1}{|\mathbf{r}_i-\mathbf{r}_j|}+\sum_{i=1}^{N} v(\mathbf{r}_i)\Bigg\}d\mathbf{r}_1\dots d\mathbf{r}_N.\eqno{(3.2.6)}$$
Let $\Omega\subset\mathbb{R}^d$ be the spatial domain for one electron. Here, we consider $\Omega$ is compact and $v(\mathbf{r})\in C^\infty(\Omega)$. $W$ is defined as
$$W := \min_{\substack{{\{\mathbf{r}_i\}}\subset\Omega}}
\Bigg\{\sum_{i=1}^{N-1}\sum_{j=i+1}^N \frac{1}{|\mathbf{r}_i-\mathbf{r}_j|}+\sum_{i=1}^{N} v(\mathbf{r}_i)\Bigg\},\eqno{(3.2.7)}$$
then                          $$E_0[\rho]\geq  \int |\Psi^{\mathrm{SCE}}(\mathbf{r}_1,\dots,\mathbf{r}_N)|^2Wd\mathbf{r}_1\dots d\mathbf{r}_N =W.\eqno{(3.2.8)}$$
If we assume ${\{\tilde{\mathbf{r}}_i\}}_{i=1}^N\in U$, where
$$U := \{\{\mathbf{r}_i\}_{i=1}^N\subset\Omega^N|\{\mathbf{r}_i\}_{i=1}^N \,\, \mathrm{are \,\, minimizers \,\, of} \,\, W\},$$
and there is a $\tilde{\Psi}$ that satisfies 
$$|\tilde{\Psi}(\mathbf{r}_1,\dots,\mathbf{r}_N)|^2=\dfrac{1}{N!}\sum_{P}\delta(\mathbf{r}_1-\tilde{\mathbf{r}}_{P(1)})\times\dots\times\delta(\mathbf{r}_N-\tilde{\mathbf{r}}_{P(N)}),$$
$\tilde{\rho}$ is the corresponding density. It follows that

\begin{equation}
	\begin{aligned}                                                                                       
		E_0[\tilde{\rho}]\leq&\int|\tilde{\Psi}(\mathbf{r}_1,\dots,\mathbf{r}_N)|^2\Bigg\{\sum_{i=1}^{N-1}\sum_{j=i+1}^N \frac{1}{|\mathbf{r}_i-\mathbf{r}_j|}+\sum_{i=1}^{N} v(\mathbf{r}_i)\Bigg\}d\mathbf{r}_1\dots d\mathbf{r}_N\notag\\
		=&\sum_{i=1}^{N-1}\sum_{j=i+1}^N \frac{1}{|\tilde{\mathbf{r}}_i-\tilde{\mathbf{r}}_j|}+\sum_{i=1}^{N} v(\tilde{\mathbf{r}}_i)\\
		=&W,
	\end{aligned}
\end{equation}
then $$E_0=E_0[\tilde{\rho}]=W. \eqno{(3.2.9)}$$
The conclusion is that the minimizers ${\{\tilde{\mathbf{r}}_i\}}_{i=1}^N$ are the positions of density peaks in the SCE system.
